# Supplementary material for: HypeR: Hypothetical Reasoning With What-If and How-To Queries Using a Probabilistic Causal Approach
Source: arXiv:2203.14692 source file (2022-03-28)
Supplement: Supplementary file 1 [file oldappendix.tex]

\onecolumn
\section{Computation of What-If Queries}
\amir{what is the formal algorithm here assuming we run on the entire DB?}
\amir{what is the motivation for looking at blocks? why is the computation of what-if queries exponential in the DB size? prove}
In this section, we discuss the computation of hypothetical what-if queries. We assume that the database $D$ is associated with a PRCM $P$ that defines the probability distribution over $PWD(D)$ after a given hypothetical update $U = u_{R, B, f, S}$. 
We can also marginalize the distribution over $PWD(D)$, given an intervention, to get a distribution and a set of possible worlds for any subset of tuples $B\subseteq D$, $PWD_B$, where $PWD_B$ are all instances where all tuples $t' \notin B$ remain unchanged and all attributes of $t\in B$ can get all possible values from their respective domains \sr{B is update attribute, change $B$ to $D'$, change $B_1, B_2$ to $D_1, D_2$ etc. This is not marginalization, can use restricted to B ----- $PWD(B) \subseteq D$, and use $PWD(...)$ instead of subscript}.
The set $B$ is referred to as a \emph{block} \sr{which set? any subset of D?}. For this analysis, we consider a block decomposition of $D$, denoted by $\mathcal{B}_D=\{B_1,\cdots,B_k\}$ where $B_i\cap B_j = \phi, \forall i\neq j$ and $\cup B_i = D$, where tuples in different blocks are independent. 
We leverage the following properties to calculate the query output.

\begin{enumerate}
    \item $\sum_{I\in PWD} \Pr(I) = 1$ and $\sum_{I'\in PWD_B} \Pr(I') = 1$, i.e., the sum of probabilities for all possible worlds of a database or a tuple is 1 \sr{tuple is not mentioned.. database and subset mentioned}.
    \item Consider a partitioning of $D$ into non-overlapping blocks $\mathcal{B}_D=\{B_1,\cdots,B_k\}$. $PWD$ is the same as the Cartesian product of $\overline{PWD}_B, \forall B\in \mathcal{B}_D$, where $\overline{PWD}_B$ contains all instances from $PWD_B$ restricted to tuples in $B$. Mathematically, $\overline{PWD}_B = \{I\cap B,~\forall I\in PWD_B\}$  where $I\cap B = \{t: t\in I, t.ID=t'.ID \text{ for some }t'\in B\}$. \sr{why not define PWD(B) directly as possible worlds of B without mentioning other tuples?}
    \item If the tuples in different blocks of the database are independent, then $\Pr(I) = \prod\limits_{I'\in PWD_B, \forall B\in \mathcal{B}_D} \Pr(I') $ \sr{use $\Pr(I) = \prod\limits_{B\in \mathcal{B}_D}\prod\limits_{I'\in PWD_B} \Pr(I') $}
\end{enumerate} 

%\noindent \textbf{Block-level decomposition.}
%\sg{talk about blocks here and corresponding properties}
We now present a lemma that simplifies the output of the query by leveraging block-independence and the above-mentioned properties. In this proof, we assume that 
$f(Q,D,I) = \sum_{B\in \mathcal{B}_I} f'(Q,D,B)$ for some $f'$. All aggregates (Sum, Avg, Count) satisfy this assumption and it is crucial to decompose the query evaluation on $I$ according to the block-level decomposition. Note that $f(Q,D,B)=f'(Q,D,B)$ if $Agg$ denotes Count or Sum. Whenever $Agg=Avg$, $f'(Q,D,B)=c f(Q,D,B)$, where $c$ is a constant that can be estimated from the query $Q$. \sg{Add more discussion on f'} \sr{average is not correct... it cannot be expressed as sum of f'... we need g(f'(...))}

\begin{lemma}
Consider a query \sr{old version and restricted predicates -- remember B is update attribute, FOR clause can have arbitrary predicate with post and pre that may not be easily decomposable, and we have a USE clause augmenting with aggregates}
\begin{align*}
&Q\equiv\when&\  g(A_l)\  Then\\
&\update&(A_c)= c\\
&~\and&\\
&\select&\ Agg(\post(B))\\
&\where&\  \pre(A_j)=a_j~\and\\
&&\post(A_i) = a_i %~\and\\
%&\groupby&\  \pre(A_k), \post(A_p)
\end{align*}
and $f(Q,D,I)=Agg(\{t'.B \mid t'\in I, t\in Pre(Q,I), t'.ID=t.ID, t' \in Post(Q,I)\})$. \sr{what are pre(Q, I) and post(Q, I)?}\\ If $f(Q,D,I) = \sum_{B\in \mathcal{B}_I} f'(Q,D,B)$, then the expected output of the query $Q(D) = \sum_{B''\in \mathcal{B}_D}\expectation_{B' \in \overline{PWD}_{B''}}[f(Q, D, B')] $, where  $\expectation_{B' \in \overline{PWD}_{B''}}[f'(Q, D, B')]$ denotes the expected value of $f'$ over the post-interventional distribution of the block $B''$.
\label{lem:general}
\end{lemma}
\begin{proof}
%Let $S$ denote the subset of $D$ that satisfies $g(A_l)$.
%Expected output of the query for a group $\pre(A_k)=a_k$ and $\post(A_p)=a_p$ can be written as follows. Let $\mathcal{P}$ denote the subset of $PWD$ where $A_p=a_p$ and $A_i=a_i$ for all tuples in $S$.
The query $Q$ intervenes on all tuples $t\in D$ such that $g(t.A_l)=\texttt{True}$. As discussed in Section~\ref{sec:semantics}, we estimate the expected output by modelling the probability distribution over different instances in the possible world PWD and then evaluate query output over the instance $I$ (say $f(Q,D,I)$). To evaluate $f(Q,D,I)$, we first identify a subset $S\subseteq D$ that satisfies the pre-condition, i.e., all tuples $t$ where $t.A_j=a_j$. Therefore $S=\{t: t\in D, t.A_j = a_j\}$. Now, we consider the corresponding set of tuples in $I$ to evaluate the aggregate over $B$ only for the tuples that satisfy the $\post$ condition as 
 $f(Q,D,I) = Agg(\{t'.B \text{ such that }t'\in I, t\in S, t'.ID=t.ID, t'.A_i=a_i\})$. Under this notation, we calculate the query output as follows.

%\begin{align}
%  E[Q,D] &= \sum_{I\in PWD}Pr(I_{A_c \gets c}|g(D.A_l) = True) f(D,I)
%\end{align}

%$PWD = PWD_{n, Dom, schema}$
\begin{align}
  Q(D) &= E_{Pr(I_{D.A_c \gets c \ | \ g(D.A_l) = True})}[f(Q,D, I)] =  \sum_{I\in PWD}Pr(I_{D.A_c \gets c}|g(D.A_l) = True) f(Q,D, I)\\
\end{align}

Using the assumption that $f(Q,D,I) = \sum_{B\in \mathcal{B}_I} f'(Q,D,B)$, we get the following.
\begin{align}
\scriptsize
  Q(D) &= \sum_{I\in PWD(D)}\left(\pr(I_{D.A_c \gets c|g(D.A_l) = True}) \sum_{B'\in \mathcal{B}_I} f'(Q,D,B')\right)
 \end{align}
 
 Assuming block-level independence, we substitute $\pr(I_{D.A_c \gets c|g(D.A_l) = True})=\prod_{B\in \mathcal{B}_I} \pr(B_{D.A_c \gets c|g(D.A_l) = True})$
 
 \begin{align}
  &=\sum_{I\in PWD(D)}\left(\left(\prod_{B\in \mathcal{B}_I} \pr(B_{D.A_c \gets c|g(D.A_l) = True})\right)  \left( \sum_{B'\in \mathcal{B}_I} f'(Q,D,B')\right)\right)\\
 &=\sum_{I\in PWD(D)} \sum_{B'\in \mathcal{B}_I}\left(\left(\prod_{B\in \mathcal{B}_I} \pr(B_{D.A_c \gets c|g(D.A_l) = True})\right) f'(Q,D,B')\right)
 \end{align}
 
 Separating out $\pr(B'_{D.A_c \gets c|g(D.A_l) = True})$ from $\prod_{B\in \mathcal{B}_I} \pr(B_{D.A_c \gets c|g(D.A_l) = True})$, we get the following.
 \begin{align}
  &=\sum_{I\in PWD(D)} \sum_{B'\in \mathcal{B}_I}\left(\left(\prod_{B\in \mathcal{B}_I\setminus\{B'\}} \pr(B_{D.A_c \gets c|g(D.A_l) = True})\right) \pr(B'_{D.A_c \gets c|g(D.A_l) = True}) f'(Q,D,B')\right)\\
  &\text{Since $B'\in \mathcal{B}_I$ is the post interventional block corresponding $B''\in \mathcal{B}_D$ where $B'.ID=B''.ID$}\\
 &=\sum_{I\in PWD(D)} \sum_{\substack{B''\in \mathcal{B}_D,\\B'\in \mathcal{B}_I  \text{such that} \\ B'.ID=B''.ID }}\left(\left(\prod_{B\in \mathcal{B}_I\setminus\{B'\}}\pr(B_{D.A_c \gets c|g(D.A_l) = True})\right) \pr(B'_{D.A_c \gets c|g(D.A_l) = True}) f'(Q,D,B')\right)\\
 &\text{Separating the second summation into two parts, $\sum_{\substack{B''\in \mathcal{B}_D,\\B'\in \mathcal{B}_I  \text{such that} \\ B'.ID=B''.ID }} \equiv \sum_{B''\in \mathcal{B}_D}\sum_{B'\in \mathcal{B}_I}\mathbbm{1}\{B'.ID=B''.ID\} $, where $\mathbbm{1}$ denotes indicator function}\\
  &=\sum_{I\in PWD(D)} \sum_{B''\in \mathcal{B}_D}\left(\sum_{B'\in \mathcal{B}_I}\mathbbm{1}\{B'.ID=B''.ID\}\left(\left(\prod_{B\in \mathcal{B}_I\setminus\{B'\}}\pr(B_{D.A_c \gets c|g(D.A_l) = True})\right) \pr(B'_{D.A_c \gets c|g(D.A_l) = True}) f'(Q,D,B')\right)\right)\\
  &\text{Swapping the two summations as $\sum_{I\in PWD(D)} $ and $\sum_{B''\in \mathcal{B}_D}$ are independent of each other}\\
&=\sum_{B''\in \mathcal{B}_D}\sum_{I\in PWD(D)} \left(\sum_{B'\in \mathcal{B}_I}\mathbbm{1}\{B'.ID=B''.ID\}\left(\left(\prod_{B\in \mathcal{B}_I\setminus\{B'\}}\pr(B_{D.A_c \gets c|g(D.A_l) = True})\right) \pr(B'_{D.A_c \gets c|g(D.A_l) = True}) f'(Q,D,B')\right)\right)
\end{align}

Substituting $PWD(D)$ as the Cartesian product of $\overline{PWD}_B$ over blocks, $PWD(D)= \bigtimes_{B\in \mathcal{B}_D} \overline{PWD}_B$
\begin{align}
&=\sum_{B''\in \mathcal{B}_D}\sum_{\substack{I\in \bigtimes_{B\in \mathcal{B}_D}  \overline{PWD}_B}} \left(\sum_{B'\in \mathcal{B}_I}\mathbbm{1}\{B'.ID=B''.ID\}\left(\left(\prod_{B\in \mathcal{B}_I\setminus\{B'\}}\pr(B_{D.A_c \gets c|g(D.A_l) = True})\right) \pr(B'_{D.A_c \gets c|g(D.A_l) = True}) f'(Q,D,B')\right)\right)
\end{align}

Substituting ${\bigtimes_{B\in \mathcal{B}_D}  \overline{PWD}_B} =  \overline{PWD}_{B''}\times \left(\bigtimes_{B\in \mathcal{B}_D\setminus \{B''\}}  \overline{PWD}_B\right)$

\begin{align}
&=\sum_{B''\in \mathcal{B}_D}\sum_{\substack{I\in\overline{PWD}_{B''}\times \\\left(\bigtimes_{B\in \mathcal{B}_D\setminus \{B''\}}  \overline{PWD}_B\right) }} \left(\sum_{B'\in \mathcal{B}_I}\mathbbm{1}\{B'.ID=B''.ID\}\left(\left(\prod_{B\in \mathcal{B}_I\setminus\{B'\}}\pr(B_{D.A_c \gets c|g(D.A_l) = True})\right) \pr(B'_{D.A_c \gets c|g(D.A_l) = True}) f'(Q,D,B')\right)\right)
\end{align}
Let $I=I'\cup I''$ where $I'\in \overline{PWD}_{B''}$ and $I''\in \left(\bigtimes_{B\in \mathcal{B}_D\setminus \{B''\}}  \overline{PWD}_B\right)$.

\begin{align}
&=\sum_{B''\in \mathcal{B}_D}\sum_{\substack{I'\in\overline{PWD}_{B''} }}\sum_{\substack{I''\in\left(\bigtimes_{B\in \mathcal{B}_D\setminus \{B''\}}  \overline{PWD}_B\right) }} \left(\sum_{B'\in \mathcal{B}_I}\mathbbm{1}\{B'.ID=B''.ID\}\left(\left(\prod_{B\in \mathcal{B}_I\setminus\{B'\}}\pr(B_{D.A_c \gets c|g(D.A_l) = True})\right) \pr(B'_{D.A_c \gets c|g(D.A_l) = True}) f'(Q,D,B')\right)\right)
\end{align}

 $I'$ corresponds to the post-intervention block of tuples in $B''$, implying $\sum_{B'\in \mathcal{B}_I}\mathbbm{1}\{B'.ID=B''.ID\}$ in the equation ensures that the indicator variable is $1$ whenever $B'=I'$.  Therefore, we replace $B'$ with $I'$.
\begin{align}
&=\sum_{B''\in \mathcal{B}_D}\sum_{\substack{I'\in\overline{PWD}_{B''} }}\sum_{\substack{I''\in\left(\bigtimes_{B\in \mathcal{B}_D\setminus \{B''\}}  \overline{PWD}_B\right) }} \left(\left(\prod_{B\in \mathcal{B}_I\setminus\{I'\}}\pr(B_{D.A_c \gets c|g(D.A_l) = True})\right) \pr(I'_{D.A_c \gets c|g(D.A_l) = True}) f'(Q,D,I')\right)
\end{align}

Separating out the terms that depend on $B''$ and $I'$ from the rest.
\begin{align}
&=\sum_{B''\in \mathcal{B}_D}\sum_{\substack{I'\in\overline{PWD}_{B''} }}\left(\left(\pr(I'_{D.A_c \gets c|g(D.A_l) = True}) f'(Q,D,I')\right)\sum_{\substack{I''\in\left(\bigtimes_{B\in \mathcal{B}_D\setminus \{B''\}}  \overline{PWD}_B\right) }} \left(\prod_{B\in \mathcal{B}_I\setminus\{I'\}}\pr(B_{D.A_c \gets c|g(D.A_l) = True})\right) \right)
\end{align}

Blocks $B\in \mathcal{B}_I\setminus\{I'\}$ are independent. Therefore, $\left(\prod_{B\in \mathcal{B}_I\setminus\{I'\}}\pr(B_{D.A_c \gets c|g(D.A_l) = True})\right)=\pr(I''_{D.A_c \gets c|g(D.A_l) = True})$
\begin{align}
&=\sum_{B''\in \mathcal{B}_D}\sum_{\substack{I'\in\overline{PWD}_{B''} }}\left(\left(\pr(I'_{D.A_c \gets c|g(D.A_l) = True}) f'(Q,D,I')\right)\sum_{\substack{I''\in\left(\bigtimes_{B\in \mathcal{B}_D\setminus \{B''\}}  \overline{PWD}_B\right) }} \left(\pr(I''_{D.A_c \gets c|g(D.A_l) = True})\right) \right)\\
&\text{Since $\sum_{\substack{I''\in\left(\bigtimes_{B\in \mathcal{B}_D\setminus \{B''\}}  \overline{PWD}_B\right) }} \left(\pr(I''_{D.A_c \gets c|g(D.A_l) = True})\right)$ is $1$}\\
&=\sum_{B''\in \mathcal{B}_D}\sum_{\substack{I'\in\overline{PWD}_{B''} }}\left(\pr(I'_{D.A_c \gets c|g(D.A_l) = True}) f'(Q,D,I')\right) 
\end{align}
Notice that the term $\sum_{\substack{I'\in\overline{PWD}_{B''} }}\left(\pr(I'_{D.A_c \gets c|g(D.A_l) = True}) f'(Q,D,I')\right) $ denotes the expected value of $f'$ over the post-interventional distribution, denoted by $\expectation_{B' \in \overline{PWD}_{B''}}[f'(Q, D, B')]$.
\end{proof}

Benefit of Lemma~\ref{lem:general}, suppose Agg  is count(*). Then $f(Q,D,I) = f'(Q,D,I) = \sum_{t'\in I,t\in D |t.ID=t'.ID} \mathbbm{1}\{t.A_j=a_j, t'.A_i=ai\}$.

Therefore, query output is $\Pr(A_i=a_i | A_j=a_j, \Do(A_c)=c)$ under independence assumptions, homogeneity and $A_c\cap (A_i\cup A_j) = \phi$.

\sg{We can show similar simplification for all aggregates.}

\begin{lemma}
Consider a query 
\begin{align*}
&Q\equiv\when&\  g(A_l)\  Then\\
&\update&(A_c)= c\\
&~\and&\\
&\select&\ Count(*)\\
&\where&\  \pre(A_j)=a_j~\and\\
&&\post(A_i) = a_i %~\and\\
%&\groupby&\  \pre(A_k), \post(A_p)
\end{align*}
then the expected output of the query $Q(D) =  |D| \pr(A_i=a_i|A_c\leftarrow c, A_j=a_j, g(A_j)) + \sum_{t\in D}\mathbbm{1}\{t.A_j=a_j, t\notin g(D.A_j), t.A_i=a_i\} $
\end{lemma}
\begin{proof}
For this query, Agg=Count and $B=*$.  Therefore,
\begin{align}
    f(Q,D,I) &= \sum_{t\in D,t'\in I} \mathbbm{1}\{t.A_j=a_j, t'.ID=t.ID, t'.A_i=a_i\}\\
    &=\sum_{t'\in I}\sum_{t\in D} \mathbbm{1}\{  t.A_j=a_j, t'.ID=t.ID, t'.A_i=a_i\}\\
     &=\sum_{B\in \mathcal{B}_I}\sum_{t'\in B}\sum_{t\in D} \mathbbm{1}\{ t.A_j=a_j, t'.ID=t.ID, t'.A_i=a_i\}\\
      &=\sum_{B\in \mathcal{B}_I}\sum_{t'\in B,t\in D} \mathbbm{1}\{  t.A_j=a_j, t'.ID=t.ID, t'.A_i=a_i\}\\
     &=\sum_{B\in \mathcal{B}_I} f(Q,D,B)
\end{align}
Using Lemma~\ref{}, $Q(D)$ is simplified as follows.\\
%\begin{align}
%Q(D)&=\sum_{B''\in \mathcal{B}_D}\sum_{\substack{I'\in\overline{PWD}_{B''} }}\left(\pr(I'_{D.A_c \gets c|g(D.A_l) = True}) f'(Q,D,I')\right) \\
%&=\sum_{B''\in \mathcal{B}_D} \sum_{\substack{I'\in\overline{PWD}_{B''} }}\left(\pr(I'_{D.A_c \gets c|g(D.A_l) = True}) \sum_{t\in B'',t'\in I' \mid t.ID=t'.ID}\mathbbm{1}\{t.A_j=a_j, t'.A_i=a_i\}\right) \\
%&=\sum_{t\in D} \sum_{\substack{t'\in\overline{PWD}_{t} }}\left(\pr(t'_{D.A_c \gets c|g(D.A_l) = True}) \mathbbm{1}\{t.A_j=a_j, t'.A_i=a_i\}\right) \\
%&=\sum_{t\in D}\mathbbm{1}\{t.A_j=a_j\} \sum_{\substack{t'\in\overline{PWD}_{t} }}\left(\pr(t'_{D.A_c \gets c|g(D.A_l) = True}) \mathbbm{1}\{ t'.A_i=a_i\}\right) \\
%&=\sum_{t\in D}\mathbbm{1}\{t.A_j=a_j, t\in g(D.A_j)\} \pr(t.A_i=a_i|D.A_c\leftarrow c)  + \sum_{t\in D}\mathbbm{1}\{t.A_j=a_j, t\notin g(D.A_j), t.A_i=a_i\}\\
%&=\sum_{t\in D}\mathbbm{1}\{t.A_j=a_j,t\in g(D.A_j)\} \pr(t.A_i=a_i|t.A_c\leftarrow c) + \sum_{t\in D}\mathbbm{1}\{t.A_j=a_j, t\notin g(D.A_j), t.A_i=a_i\} \\
%&= |D| \pr(A_i=a_i|A_c\leftarrow c, A_j=a_j, g(A_j)) + \sum_{t\in D}\mathbbm{1}\{t.A_j=a_j, t\notin g(D.A_j), t.A_i=a_i\} \\
%\end{align}
\begin{align}
Q(D)&=\sum_{B''\in \mathcal{B}_D}\sum_{\substack{I'\in\overline{PWD}_{B''} }}\left(\pr(I'_{D.A_c \gets c|g(D.A_l) = True}) f'(Q,D,I')\right) \\
&=\sum_{B''\in \mathcal{B}_D} \sum_{\substack{I'\in\overline{PWD}_{B''} }}\left(\pr(I'_{D.A_c \gets c|g(D.A_l) = True}) \sum_{t\in B'',t'\in I' \mid t.ID=t'.ID}\mathbbm{1}\{t.A_j=a_j, t'.A_i=a_i\}\right) \\
&=\sum_{B''\in \mathcal{B}_D} \sum_{\substack{I'\in\overline{PWD}_{B''} }}\left(\pr(I'_{D.A_c \gets c|g(D.A_l) = True}) \sum_{t\in B''}\left(\mathbbm{1}\{t.A_j=a_j\}\mathbbm{1}\{t'.A_i=a_i, \text{where } t'.ID=t.ID, t'\in I'\}\right)\right) \\
&=\sum_{B''\in \mathcal{B}_D}\left(\sum_{t\in B''}\left(\mathbbm{1}\{t.A_j=a_j\} \sum_{\substack{I'\in\overline{PWD}_{B''} }}\left(\pr(I'_{D.A_c \gets c|g(D.A_l) = True}) \sum_{t'\in I' \mid t.ID=t'.ID}\mathbbm{1}\{ t'.A_i=a_i\}\right)\right)\right) \sg{same as 34}\\
&=\sum_{B''\in \mathcal{B}_D}\left(\sum_{t\in B''}\mathbbm{1}\{t.A_j=a_j\}\sum_{t''\in B'' }\left( \sum_{\substack{I'\in\overline{PWD}_{B''}\\ t'\in I', t''.ID=t'.ID=t.ID} }\left(\pr(I'_{D.A_c \gets c|g(D.A_l) = True}) \mathbbm{1}\{ t'.A_i=a_i\}\right)\right)\right) \\
&\text{Innermost summation is non-zero only when $t''=t$}\\
&=\sum_{B''\in \mathcal{B}_D}\left(\sum_{t\in B''}\mathbbm{1}\{t.A_j=a_j\}\left( \sum_{\substack{I'\in\overline{PWD}_{B''}\\ t'\in I', t.ID=t'.ID} }\left(\pr(I'_{D.A_c \gets c|g(D.A_l) = True}) \mathbbm{1}\{ t'.A_i=a_i\}\right)\right)\right) \\
%&=\sum_{B''\in \mathcal{B}_D}\left(\sum_{t\in B''}\mathbbm{1}\{t.A_j=a_j\} \left(\sum_{t''\in B'',t''.ID=t.ID} \pr(t''.A_i=a_i| D.A_c{g(D.A_l)=True}\gets c)\right)\right) \\
&=\sum_{B''\in \mathcal{B}_D}\left(\sum_{t\in B''} \left( \pr(t.A_i=a_i| t.A_j=a_j, t''.A_c\leftarrow c, \  \forall t''\in B''\cap g(D.A_l))\right)\right) \end{align}
We now use backdoor criterion to estimate the probability values from the original database $D$.

\begin{align}
&\sg{can we have a better notation for the above equation}\\
&=\sum_{B''\in \mathcal{B}_D}\sum_{c\in \Dom (C_{B''})}\left(\sum_{t\in B''} \left( \pr(t.A_i=a_i| t.A_j=a_j, t''.A_c= c, \  \forall t''\in B''\cap g(D.A_l), C_{B''}=c)\right) \pr(c|t.A_j=a_j)\right) \\
\end{align}

\end{proof}

\clearpage
\onecolumn
\section{Extension: Computation of What-If Queries}

{Generalization: Let $f(Q,D,I) =g( f'(Q,D,B_1),\ldots,f'(Q,D,B_t))$.
Assumption: g is homogenous to degree 1 and f is composable.}

\begin{assumption}We make the following assumptions:\\
\begin{itemize}
    \item $f(Q,D,I) = g(\{f'(Q,D,B) \forall B\in \mathcal{B}_I\})$
    \item $\alpha g(\{x_1,\ldots,x_t\}) = g(\{\alpha x_1,\ldots,\alpha x_t\})$, $\alpha \geq 0$
    \item $ g(\{x_1,\ldots,x_t\}) + g(\{y_1,\ldots,y_t\}) = g(\{x_1+y_1,\ldots, x_t+y_t\})$
\end{itemize}\label{assume:homogenous}
\end{assumption}

\begin{lemma}
Consider a query 
\begin{align*}
&Q\equiv\when&\  g(A_l)\  Then\\
&\update&(A_c)= c\\
&~\and&\\
&\select&\ Agg(\post(B))\\
&\where&\  \pre(A_j)=a_j~\and\\
&&\post(A_i) = a_i %~\and\\
%&\groupby&\  \pre(A_k), \post(A_p)
\end{align*}
and $f(Q,D,I)=Agg(\{t'.B \mid t'\in I, t\in Pre(Q,I), t'.ID=t.ID, t' \in Post(Q,I)\})$.\\ If Agg satisfies the assumption~\ref{assume:homogenous}, then the expected output of the query $Q(D) = g\left(\left\{\expectation_{B' \in \overline{PWD}_{B''}}[f(Q, D, B')] \forall B''\in \mathcal{B}_D\right\}\right)$.
\label{lem:general}
\end{lemma}
\begin{proof}
%Let $S$ denote the subset of $D$ that satisfies $g(A_l)$.
%Expected output of the query for a group $\pre(A_k)=a_k$ and $\post(A_p)=a_p$ can be written as follows. Let $\mathcal{P}$ denote the subset of $PWD$ where $A_p=a_p$ and $A_i=a_i$ for all tuples in $S$.
The query $Q$ intervenes on all tuples $t\in D$ such that $g(t.A_l)=\texttt{True}$. As discussed in Section~\ref{sec:semantics}, we estimate the expected output by modelling the probability distribution over different instances in the possible world PWD and then evaluate query output over the instance $I$ (say $f(Q,D,I)$). To evaluate $f(Q,D,I)$, we first identify a subset $S\subseteq D$ that satisfies the pre-condition, i.e., all tuples $t$ where $t.A_j=a_j$. Therefore $S=\{t: t\in D, t.A_j = a_j\}$. Now, we consider the corresponding set of tuples in $I$ to evaluate the aggregate over $B$ only for the tuples that satisfy the $\post$ condition as 
 $f(Q,D,I) = Agg(\{t'.B \text{ such that }t'\in I, t\in S, t'.ID=t.ID, t'.A_i=a_i\})$. Under this notation, we calculate the query output as follows.

%\begin{align}
%  E[Q,D] &= \sum_{I\in PWD}Pr(I_{A_c \gets c}|g(D.A_l) = True) f(D,I)
%\end{align}

%$PWD = PWD_{n, Dom, schema}$
\begin{align}
  Q(D) &= E_{Pr(I_{D.A_c \gets c \ | \ g(D.A_l) = True})}[f(Q,D, I)] =  \sum_{I\in PWD}Pr(I_{D.A_c \gets c}|g(D.A_l) = True) f(Q,D, I)\\
\end{align}

Using the assumption that $f(Q,D,I) = \sum_{B\in \mathcal{B}_I} f'(Q,D,B)$, we get the following.
\begin{align}
\scriptsize
  Q(D) &= \sum_{I\in PWD_D}\left(\pr(I_{D.A_c \gets c|g(D.A_l) = True}) g(\{ f'(Q,D,B'), \forall B'\in \mathcal{B}_I\})\right)
 \end{align}
 Assuming block-level independence, we substitute $\pr(I_{D.A_c \gets c|g(D.A_l) = True})=\prod_{B\in \mathcal{B}_I} \pr(B_{D.A_c \gets c|g(D.A_l) = True})$
 
 \begin{align}
  &=\sum_{I\in PWD_D}\left(\left(\prod_{B\in \mathcal{B}_I} \pr(B_{D.A_c \gets c|g(D.A_l) = True})\right)  \left( g(\{ f'(Q,D,B'), \forall B'\in \mathcal{B}_I\})\right)\right)\\
 &=\sum_{I\in PWD_D} g\left(\left\{\left(\prod_{B\in \mathcal{B}_I} \pr(B_{D.A_c \gets c|g(D.A_l) = True})\right) f'(Q,D,B') \forall B'\in \mathcal{B}_I\right\}\right)
 \end{align}
 
 Separating out $\pr(B'_{D.A_c \gets c|g(D.A_l) = True})$ from $\prod_{B\in \mathcal{B}_I} \pr(B_{D.A_c \gets c|g(D.A_l) = True})$, we get the following.
 \begin{align}
  &=\sum_{I\in PWD_D} g\left(\{\left(\prod_{B\in \mathcal{B}_I\setminus\{B'\}} \pr(B_{D.A_c \gets c|g(D.A_l) = True})\right) \pr(B'_{D.A_c \gets c|g(D.A_l) = True}) f'(Q,D,B') \forall B'\in \mathcal{B}_I\}\right)\\
  &\text{Since $B'\in \mathcal{B}_I$ is the post interventional block corresponding $B''\in \mathcal{B}_D$ where $B'.ID=B''.ID$}\\
 &=\sum_{I\in PWD_D} g \left\{\sum_{\substack{B''\in \mathcal{B}_D,\\ \text{such that} \\ B'.ID=B''.ID }} \left(\left(\prod_{B\in \mathcal{B}_I\setminus\{B'\}}\pr(B_{D.A_c \gets c|g(D.A_l) = True})\right) \pr(B'_{D.A_c \gets c|g(D.A_l) = True}) f'(Q,D,B')\right), \forall B'\in \mathcal{B}_I\right\}\\
 %&\text{Separating the second summation into two parts, $\sum_{\substack{B''\in \mathcal{B}_D,\\B'\in \mathcal{B}_I  \text{such that} \\ B'.ID=B''.ID }} \equiv \sum_{B''\in \mathcal{B}_D}\sum_{B'\in \mathcal{B}_I}\mathbbm{1}\{B'.ID=B''.ID\} $, where $\mathbbm{1}$ denotes indicator function}\\
  &=\sum_{I\in PWD_D}g\left\{ \left(\sum_{B'\in \mathcal{B}_I}\mathbbm{1}\{B'.ID=B''.ID\}\left(\left(\prod_{B\in \mathcal{B}_I\setminus\{B'\}}\pr(B_{D.A_c \gets c|g(D.A_l) = True})\right) \pr(B'_{D.A_c \gets c|g(D.A_l) = True}) f'(Q,D,B')\right)\right), \forall B''\in\mathcal{B}_D\right\}\\
&=g\left\{\sum_{I\in PWD_D} \left(\sum_{B'\in \mathcal{B}_I}\mathbbm{1}\{B'.ID=B''.ID\}\left(\left(\prod_{B\in \mathcal{B}_I\setminus\{B'\}}\pr(B_{D.A_c \gets c|g(D.A_l) = True})\right) \pr(B'_{D.A_c \gets c|g(D.A_l) = True}) f'(Q,D,B')\right)\right), \forall B''\in \mathcal{B}_D\right\}
\end{align}

Substituting $PWD_D$ as the Cartesian product of $\overline{PWD}_B$ over blocks, $PWD_D= \bigtimes_{B\in \mathcal{B}_D} \overline{PWD}_B$
\begin{align}
&=g\left\{\sum_{\substack{I\in \bigtimes_{B\in \mathcal{B}_D}  \overline{PWD}_B}} \left(\sum_{B'\in \mathcal{B}_I}\mathbbm{1}\{B'.ID=B''.ID\}\left(\left(\prod_{B\in \mathcal{B}_I\setminus\{B'\}}\pr(B_{D.A_c \gets c|g(D.A_l) = True})\right) \pr(B'_{D.A_c \gets c|g(D.A_l) = True}) f'(Q,D,B')\right)\right),\forall B''\in \mathcal{B}_D\right\}
\end{align}

Substituting ${\bigtimes_{B\in \mathcal{B}_D}  \overline{PWD}_B} =  \overline{PWD}_{B''}\times \left(\bigtimes_{B\in \mathcal{B}_D\setminus \{B''\}}  \overline{PWD}_B\right)$

\begin{align}
&=g\left\{\sum_{\substack{I\in\overline{PWD}_{B''}\times \\\left(\bigtimes_{B\in \mathcal{B}_D\setminus \{B''\}}  \overline{PWD}_B\right) }} \left(\sum_{B'\in \mathcal{B}_I}\mathbbm{1}\{B'.ID=B''.ID\}\left(\left(\prod_{B\in \mathcal{B}_I\setminus\{B'\}}\pr(B_{D.A_c \gets c|g(D.A_l) = True})\right) \pr(B'_{D.A_c \gets c|g(D.A_l) = True}) f'(Q,D,B')\right)\right), \forall {B''\in \mathcal{B}_D}\right\}
\end{align}
Let $I=I'\cup I''$ where $I'\in \overline{PWD}_{B''}$ and $I''\in \left(\bigtimes_{B\in \mathcal{B}_D\setminus \{B''\}}  \overline{PWD}_B\right)$.

\begin{align}
&=g\left\{\sum_{\substack{I'\in\overline{PWD}_{B''} }}\sum_{\substack{I''\in\left(\bigtimes_{B\in \mathcal{B}_D\setminus \{B''\}}  \overline{PWD}_B\right) }} \left(\sum_{B'\in \mathcal{B}_I}\mathbbm{1}\{B'.ID=B''.ID\}\left(\left(\prod_{B\in \mathcal{B}_I\setminus\{B'\}}\pr(B_{D.A_c \gets c|g(D.A_l) = True})\right) \pr(B'_{D.A_c \gets c|g(D.A_l) = True}) f'(Q,D,B')\right)\right),{B''\in \mathcal{B}_D}\right\}
\end{align}

 $I'$ corresponds to the post-intervention block of tuples in $B''$, implying $\sum_{B'\in \mathcal{B}_I}\mathbbm{1}\{B'.ID=B''.ID\}$ in the equation ensures that the indicator variable is $1$ whenever $B'=I'$.  Therefore, we replace $B'$ with $I'$.
\begin{align}
&=g\left\{\sum_{\substack{I'\in\overline{PWD}_{B''} }}\sum_{\substack{I''\in\left(\bigtimes_{B\in \mathcal{B}_D\setminus \{B''\}}  \overline{PWD}_B\right) }} \left(\left(\prod_{B\in \mathcal{B}_I\setminus\{I'\}}\pr(B_{D.A_c \gets c|g(D.A_l) = True})\right) \pr(I'_{D.A_c \gets c|g(D.A_l) = True}) f'(Q,D,I')\right), \forall {B''\in \mathcal{B}_D}\right\}
\end{align}

Separating out the terms that depend on $B''$ and $I'$ from the rest.
\begin{align}
&=g\left\{\sum_{\substack{I'\in\overline{PWD}_{B''} }}\left(\left(\pr(I'_{D.A_c \gets c|g(D.A_l) = True}) f'(Q,D,I')\right)\sum_{\substack{I''\in\left(\bigtimes_{B\in \mathcal{B}_D\setminus \{B''\}}  \overline{PWD}_B\right) }} \left(\prod_{B\in \mathcal{B}_I\setminus\{I'\}}\pr(B_{D.A_c \gets c|g(D.A_l) = True})\right) \right),\forall {B''\in \mathcal{B}_D}\right\}
\end{align}

Blocks $B\in \mathcal{B}_I\setminus\{I'\}$ are independent. Therefore, $\left(\prod_{B\in \mathcal{B}_I\setminus\{I'\}}\pr(B_{D.A_c \gets c|g(D.A_l) = True})\right)=\pr(I''_{D.A_c \gets c|g(D.A_l) = True})$
\begin{align}
&=g\left\{\sum_{\substack{I'\in\overline{PWD}_{B''} }}\left(\left(\pr(I'_{D.A_c \gets c|g(D.A_l) = True}) f'(Q,D,I')\right)\sum_{\substack{I''\in\left(\bigtimes_{B\in \mathcal{B}_D\setminus \{B''\}}  \overline{PWD}_B\right) }} \left(\pr(I''_{D.A_c \gets c|g(D.A_l) = True})\right) \right), {B''\in \mathcal{B}_D}\right\}\\
&\text{Since $\sum_{\substack{I''\in\left(\bigtimes_{B\in \mathcal{B}_D\setminus \{B''\}}  \overline{PWD}_B\right) }} \left(\pr(I''_{D.A_c \gets c|g(D.A_l) = True})\right)$ is $1$}\\
&=g\{\sum_{\substack{I'\in\overline{PWD}_{B''} }}\left(\pr(I'_{D.A_c \gets c|g(D.A_l) = True}) f'(Q,D,I')\right),\forall B''\in \mathcal{B}_D \}
\end{align}
Notice that the term $\sum_{\substack{I'\in\overline{PWD}_{B''} }}\left(\pr(I'_{D.A_c \gets c|g(D.A_l) = True}) f'(Q,D,I')\right) $ denotes the expected value of $f'$ over the post-interventional distribution, denoted by $\expectation_{B' \in \overline{PWD}_{B''}}[f(Q, D, B')]$.
\end{proof}

\clearpage

Generalize to percentile
-------------------
\sg{Older proofs below}

\begin{lemma}
Count query under independence assumption
\end{lemma}
\begin{proof}
Expected output of the query can be written as
\begin{align}
   &= \sum_{I\in PWD} Pr(I|\update(A_c)=c, \pre(A_j)=a_j)Q(I)\\
   &\text{Assuming independence of tuples}\\
    &=\sum_{I\in PWD} \left(\left(\prod_{t\in I}Pr(I.t)\right) Q(I)\right)\\
   &=\sum_{I\in PWD}\sum_{ t\in I} \left(\left(\prod_{t'\in I}Pr(I.t')\right) \mathbbm{1}\{{t.A_i=a_i}\}\right)\\
   &{t=\post(t_p)}\\
   &=\sum_{I\in PWD}\sum_{ \post(t_p)\in I} \left(\left(\prod_{t'\in I}Pr(I.t')\right) \mathbbm{1}\{{t.A_i=a_i}\}\right)\\
    &=\sum_{I\in PWD}\sum_{ t_p\in D} \left(\left(\prod_{t'\in I}Pr(I.t')\right) \mathbbm{1}\{{t.A_i=a_i}\}\right)\\
   &=\sum_{t_p\in D}\sum_{I\in PWD} \left(\left(\prod_{t'\in I}Pr(I.t')\right) \mathbbm{1}\{{t.A_i=a_i}\}\right)\\
   &=\sum_{t_p\in D}\sum_{I\in PWD}\left(\prod_{t'\in I,t'\neq t}Pr(I.t') \right) \left(Pr(I.t)\mathbbm{1}\{{t.A_i=a_i}\}\right)\\
   %&=\sum_{t_p\in D}\pro{t'\neq t, T.t'\in PWD(t')}\sum_{I.t\in PWD(t)} \left(Pr(I.t)\mathbbm{1}\{{t.A_i=a_i}\}\right)\\
   &=\sum_{t_p\in D}\sum_{I\in PWD(t)} \left(Pr(I)\mathbbm{1}\{{t.A_i=a_i}\}\right)\\
  &=\sum_{t_p\in D}Pr(t.A_i=a_i|\Do(A_c)=c)\\
  &=|D| Pr(A_i=a_i|\Do(A_c)=c)\\
\end{align}

\end{proof}
