# Supplementary material for: HypeR: Hypothetical Reasoning With What-If and How-To Queries Using a Probabilistic Causal Approach
Source: arXiv:2203.14692 source file (2022-03-28)
Supplement: Supplementary file 2 [file appendix.tex]

\section{Extension to Multi-attribute updates}
\sys relies on the computation of post-update probability distribution using a probabilistic Relational Causal Model. In case of a single attribute update, we leverage the backdoor criterion to estimate post-update probabilities.

\begin{align} \scriptsize
    \pr_{D, U}(Y=y \mid B=b,\mb C=\mb c )= \pr_{D}(Y=y \mid B=f(b), \mb C=\mb c )  \label{eq:back}
\end{align}

In case where multiple attributes are updated, it extends whenever the updated attributes do not have a descendant path.

\section{Preferential Multi-attribute Optimization for How-To queries }
